# Supplementary material for: Decentralized Dynamic Stable Matching
Source: arXiv:2610.41912 source file (2026-11-06)
Supplement: Supplementary file 1 [file learning-lower-bounds.tex]

\subsection{Statistical lower bounds and recovery in the learning model}
\label{app:learning-lower}

The proof of \cref{cor:learning-static-lower} combines the accepted-edge information bound in Section~\ref{sec:learning-lower:information} with the arm-side construction in Section~\ref{sec:learning-lower:arm-side}. Section~\ref{sec:learning-lower:program} develops a general information bound for the POSM objective, and Section~\ref{sec:learning-lower:one-player} gives a complementary player-side construction. Section~\ref{sec:learning-lower:recovery} combines statistical cost with hidden-departure recovery under an additional window condition. The population-prefix bound in Section~\ref{sec:learning-lower:prefix} uses a separate instance family; Section~\ref{sec:learning-lower:interpretation} compares the resulting bounds and objectives.

For the statistical bounds, we use independent Bernoulli rewards at both endpoints of each accepted edge, a subclass of the conditional-mean model. The protocol and its arm-service rules are fixed before the means are chosen; rejection supplies neither a reward observation nor an exogenous ranking oracle. These bounds hold even for a central controller that can choose any feasible matching and observe every accepted reward, and can therefore simulate every local state and decision of SC-PC. Theorem~\ref{thm:learning} makes SC-PC uniformly efficient in the sense of \cref{cor:learning-static-lower}. The recovery argument in Section~\ref{sec:learning-lower:recovery} reinstates the local information restrictions, under which departures are not announced.

\subsubsection{Information from accepted edges}
\label{sec:learning-lower:information}

An alternative can change the POSM while preserving the reward laws on every original POSM edge. Distinguishing such an alternative requires observations from other edges. We first express the information in those observations.

\paragraph{Transcript divergence.}
Let $\theta$ and $\lambda$ denote two static mean instances with the same population and endpoint means $\mu_{i,x}$ and $\pi_{x,i}$, as in Section~\ref{sec:model}. Let $N_{i,x}(T)$ count acceptances of edge $(i,x)$ in the first $T$ rounds. Write $\mathbb P_\theta^T$ for the transcript law and $D_\theta(T)$ for the POSM-mismatch cost under $\theta$. Write $\operatorname{KL}$ for relative entropy and $\operatorname{kl}$ for its Bernoulli specialization, both defined using natural logarithms. On the full observation transcript, the chain rule gives
\begin{equation}
 \operatorname{KL}(\mathbb P_\theta^T,\mathbb P_\lambda^T)
 =\sum_{i,x}\mathbb E_\theta N_{i,x}(T)
 \left\{\operatorname{kl}(\mu_{i,x}^{\theta},\mu_{i,x}^{\lambda})
             +\operatorname{kl}(\pi_{x,i}^{\theta},\pi_{x,i}^{\lambda})\right\}.
\label{eq:learning-lower:kl-transcript}
\end{equation}
Conditional on the same observed history, the protocol uses the same action and state-update laws in both instances. Only the distributions of newly observed endpoint rewards can differ, so all divergence accumulates through these observations. Rejections and local state transitions contribute no additional term. Equation \eqref{eq:learning-lower:kl-transcript} specializes the adaptive change-of-measure identity to two observations per accepted edge; see also \cite[Lemma 1]{KCG16}.

\paragraph{One-edge alternatives.}
Suppose edge $e$ is absent from the original POSM and present in the alternative POSM, and the two instances differ only in one endpoint mean on that edge, which changes from $p$ to $q$. Then
\[
              N_e(T)\le D_\theta(T),\qquad
              T-N_e(T)\le D_\lambda(T)
\]
pathwise in their respective instances. For a uniformly efficient protocol and every $\alpha\in(0,1)$, the event $A_T=\{N_e(T)<T/2\}$ satisfies
\[
 \mathbb P_\theta(A_T)=1-o(T^{\alpha-1}),\qquad
 \mathbb P_\lambda(A_T)=o(T^{\alpha-1}).
\]
This follows directly from Markov's inequality and the definition of uniform efficiency. Binary data processing and the bound on binary entropy imply
\[
 \operatorname{KL}(\mathbb P_\theta^T,\mathbb P_\lambda^T)
 \ge \mathbb P_\theta(A_T)\ln\frac1{\mathbb P_\lambda(A_T)}-\ln2.
\]
Divide by $\ln T$, take the lower limit, and then let $\alpha\downarrow0$. Using \eqref{eq:learning-lower:kl-transcript}, we obtain
\begin{equation}
 \liminf_{T\to\infty}\frac{\mathbb E_\theta N_e(T)}{\ln T}
                 \ge\frac1{\operatorname{kl}(p,q)}.
\label{eq:learning-lower:one-edge}
\end{equation}
Under this one-edge perturbation, the argument requires only a change in POSM membership; uniqueness of the stable matching is unnecessary. It also remains valid when the unchanged means are revealed to the controller. The constructions in Sections~\ref{sec:learning-lower:arm-side} and \ref{sec:learning-lower:one-player} will use instances with unique stable matchings.

\subsubsection{An information bound for the player-optimal objective}
\label{sec:learning-lower:program}

We now collect the information constraints into a lower bound for the POSM objective. Fix the population and consider the full class of Bernoulli instances with strict preferences and means in $(0,1)$. Uniform efficiency is required throughout this class. For an edge $e=(i,x)$, write $\mu_e=\mu_{i,x}$ and $\pi_e=\pi_{x,i}$. Let $\mathcal M$ be the finite set of feasible partial matchings and define
\[
 k_e(\theta,\lambda)=\operatorname{kl}(\mu_e^\theta,\mu_e^\lambda)+\operatorname{kl}(\pi_e^\theta,\pi_e^\lambda),
 \qquad k_M(\theta,\lambda)=\sum_{e\in M}k_e(\theta,\lambda).
\]
If $m_\lambda^*\ne m_\theta^*$, consider the event that $m_\theta^*$ is played on more than $T/2$ rounds. Uniform efficiency gives probability $1-o(T^{\alpha-1})$ under $\theta$ and $o(T^{\alpha-1})$ under $\lambda$. Applying the preceding data-processing argument yields
\begin{equation}
 \liminf_{T\to\infty}
     \frac{\operatorname{KL}(\mathbb P_\theta^T,\mathbb P_\lambda^T)}{\ln T}\ge1.
\label{eq:learning-lower:posm-kl}
\end{equation}
We focus on alternatives that change the POSM while preserving every reward law observed under the original POSM:
\[
 \mathcal A_{\mathrm{POSM}}(\theta)=
 \{\lambda:m_\lambda^*\ne m_\theta^*,\quad
                   k_e(\theta,\lambda)=0\ \text{for every }e\in m_\theta^*\}.
\]

\begin{proposition}[A structured POSM information program]
\label{prop:learning-lower:program}
Every uniformly efficient protocol satisfies
\[
       \liminf_{T\to\infty}\frac{\mathbb E_\theta D(T)}{\ln T}
                    \ge c_{\mathrm{POSM}}(\theta),
\]
where
\begin{equation}\begin{aligned}
 c_{\mathrm{POSM}}(\theta)&=\inf_{w_M\ge0}\ \sum_{M\ne m_\theta^*}w_M,\\
 \text{subject to}\quad
 &\sum_{M\ne m_\theta^*}w_M k_M(\theta,\lambda)\ge1
       \qquad\text{for every }\lambda\in\mathcal A_{\mathrm{POSM}}(\theta).
\end{aligned}\label{eq:learning-lower:program}
\end{equation}
The value is zero if the alternative set is empty and $+\infty$ if the constraints are infeasible. The proposition does not assert that this lower bound is attainable.
\end{proposition}
\begin{proof}
Let $N_M(T)$ count the rounds whose accepted matching is $M$, and put $w_M(T)=\mathbb E_\theta N_M(T)/\ln T$ for $M\ne m_\theta^*$. The sum of these weights is $\mathbb E_\theta D(T)/\ln T$. For each alternative in the specified set, playing $m_\theta^*$ contributes no divergence. Equations \eqref{eq:learning-lower:kl-transcript} and \eqref{eq:learning-lower:posm-kl} therefore give
\[
       \liminf_T\sum_{M\ne m_\theta^*}w_M(T)k_M(\theta,\lambda)\ge1.
\]
If the normalized cost has infinite lower limit, the result is immediate. Otherwise, take a sequence along which it converges to its finite lower limit. Nonnegativity bounds every coordinate along this sequence. Since $\mathcal M$ is finite, a subsequence converges coordinatewise to a nonnegative vector $w$. For each fixed alternative, the corresponding finite linear form converges as well, so $w$ satisfies its constraint. This same limiting vector is feasible for every alternative, and its objective equals the chosen lower limit.
\end{proof}

\paragraph{Comparison with binary stability.}
Basu's binary-stability program fixes the means on the union of all originally stable edges and considers alternatives with no stable matching in common with the original instance \cite[Definition 5.1 and Theorem 5.2]{basu2025super}. When the Bernoulli parameter class and the matching permissions are the same, each such alternative belongs to $\mathcal A_{\mathrm{POSM}}(\theta)$. Every original stable matching gives zero information against it. Removing the stable-matching coordinates from a feasible POSM vector therefore produces a feasible binary-stability vector with no larger objective. Under these common conditions, $c_{\mathrm{POSM}}(\theta)\ge c_{\rm binary}(\theta)$. The next two results show why this comparison can be strict.

\begin{corollary}[Positive information cost at every strict interior instance]
\label{cor:learning-lower:positive}
For a nonempty fixed population and $K\ge2$, every strict interior instance in the full two-sided unknown-mean class has $c_{\mathrm{POSM}}(\theta)>0$.
\end{corollary}
\begin{proof}
Choose a player $i$ and an arm $x\ne m_\theta^*(i)$. Increase both endpoint means on $(i,x)$ above the other means at their respective endpoints, keeping both below one. The endpoints become mutual first choices, so their pair belongs to every stable matching. The POSM changes, while all reward laws on original POSM edges remain fixed. With $k=k_{ix}(\theta,\lambda)\in(0,\infty)$, the constraint from this alternative is
\[
                 k\sum_{M:(i,x)\in M}w_M\ge1.
\]
Thus every feasible vector has objective at least $1/k>0$.
\end{proof}

\paragraph{A strict separation.}
The following two-player, two-arm example separates the information bounds: every edge belongs to a stable matching, yet meeting the POSM objective requires further information. For $0<\delta\le1/8$, let
\[
\begin{array}{c|cc}
 &0&1\\\hline
 \mu_{1,\cdot}&1/2&1/2-\delta\\
 \mu_{2,\cdot}&1/4&3/4
\end{array}
\qquad
\begin{array}{c|cc}
 &1&2\\\hline
 \pi_{0,\cdot}&1/4&3/4\\
 \pi_{1,\cdot}&3/4&1/4
\end{array}.
\]
The matching along the diagonal of the player-mean matrix is player-optimal, while the reversed matching is also stable. Their union contains every edge, so fixing all stable-edge laws leaves the binary program with no alternative and value zero. Now change only $\mu_{1,1}$ to $1/2+\varepsilon$, with $0<\varepsilon<1/4$. The reversed matching becomes uniquely stable, and the reward laws on the diagonal edges remain unchanged. Equation \eqref{eq:learning-lower:one-edge}, followed by $\varepsilon\downarrow0$, gives
\[
 \liminf_{T\to\infty}\frac{\mathbb E_\theta N_{1,1}(T)}{\ln T}
 \ge\frac1{\operatorname{kl}(1/2-\delta,1/2)}\ge\frac1{4\delta^2}.
\]
Each such acceptance incurs a POSM mismatch. In the original instance $E_1^*=\{0\}$, $E_2^*=\{1\}$, and $\Delta_{\min}=\delta$. Thus the binary program can give a zero lower bound even when meeting the POSM objective has a positive information cost. A zero value of that program does not imply that zero regret is achievable.

\subsubsection{Arm-side learning with all player means revealed}
\label{sec:learning-lower:arm-side}

\paragraph{The instance.}
With the player means revealed, uniform efficiency is required over all strict Bernoulli arm-mean instances sharing those same player means. Fix $K$ and $\Delta$ as in \cref{cor:learning-static-lower}. Let the players be $p_0,\ldots,p_{K-1}$ and the arms $0,\ldots,K-1$. Each player other than $p_0$ will form a mutual first-choice pair with a distinct arm, leaving $p_0$ its last choice. Reversing one arm's preference between its owner and $p_0$ changes the POSM; learning those comparisons will account for the lower bound. Choose player means
\[
 \mu_{p_0,j}=\frac12+(K-1-j)\Delta,
 \qquad
 \mu_{p_r,j}=\begin{cases}
       3/4,&j=r-1,\\
       1/8+(j+1)/(8K),&j\ne r-1,
      \end{cases}\qquad 1\le r<K.
\]
On each arm $j<K-1$, set
\[
 \pi_{j,p_{j+1}}=\frac12,\qquad
 \pi_{j,p_0}=\frac12-\Delta,\qquad
 \pi_{j,p_r}=\frac18+\frac r{8K}\quad(r\notin\{0,j+1\}).
\]
On the last arm, set $\pi_{K-1,p_0}=3/4$ and $\pi_{K-1,p_r}=1/8+r/(8K)$ for $r\ge1$. All means are interior and all local rankings are strict. In each pair $(p_r,r-1)$, $r\ge1$, the endpoints are mutual first choices, so the pair occurs in every stable matching. The remaining player $p_0$ receives arm $K-1$, giving a unique stable matching.

\paragraph{The relevant gap.}
For this instance,
\[
 E_{p_0}^*=\mathcal K,\qquad E_{p_r}^*=\{r-1\}\quad(r\ge1).
\]
Among the means of player $p_0$, the smallest positive difference is $\Delta$. For each other player, the reward gap between its assigned first choice and any other arm is at least $1/2$. At each arm $j$ other than the last, the only distinct players whose relevant sets both contain that arm are $p_0$ and $p_{j+1}$; the difference between their means at this arm is $\Delta$. The last arm belongs only to the remaining player's relevant set. Consequently $\Delta_{\min}=\Delta$ exactly.

\paragraph{Alternatives and information cost.}
For each $j<K-1$, change only $\pi_{j,p_0}$ to $1/2+\varepsilon$, where $0<\varepsilon<1/8$. All player means remain fixed. The endpoints of the other $K-2$ owner pairs remain mutual first choices. In the remaining market, $p_0$ prefers $j$ to $K-1$ and $j$ prefers $p_0$ to its former owner, so $(p_0,j)$ belongs to every stable matching. The displaced owner receives $K-1$, again giving a unique stable matching. For $N_j=N_{p_0,j}$, \eqref{eq:learning-lower:one-edge} implies
\[
 \liminf_{T\to\infty}\frac{\mathbb E N_j(T)}{\ln T}
       \ge\frac1{\operatorname{kl}(1/2-\Delta,1/2+\varepsilon)}.
\]
Let $\varepsilon\downarrow0$. Each acceptance of one of these edges in the original instance incurs a mismatch. Since the same player cannot be accepted at two arms in one round, $\sum_{j<K-1}N_j(T)\le D(T)$. For $p\in[3/8,1/2]$, the second derivative of $p\mapsto\operatorname{kl}(p,1/2)$ is $1/[p(1-p)]\le64/15$. Its value and first derivative vanish at $p=1/2$, so Taylor's theorem and $\Delta\le1/8$ give
\[
 \operatorname{kl}(1/2-\Delta,1/2)
 \le\frac{32}{15}\Delta^2
 <4(\ln2)\Delta^2.
\]
Converting the normalization in \eqref{eq:learning-lower:one-edge} to base two and summing therefore gives
\[
 \liminf_{T\to\infty}\frac{\mathbb E D(T)}{\log T}
 \ge\frac{(\ln2)(K-1)}{\operatorname{kl}(1/2-\Delta,1/2)}
 \ge\frac{K-1}{4\Delta^2}.
\]
All alternatives change only arm means. The construction therefore proves \cref{cor:learning-static-lower} even when all player means are revealed and accepted observations are centralized: the uncertainty responsible for the bound lies entirely on the arm side.

\subsubsection{A complementary one-player construction}
\label{sec:learning-lower:one-player}

A complementary player-side construction permits a gap range independent of the number of arms. For any $K\ge2$ and $0<\delta\le1/8$, take one permanent player $i$ with
\[
 \mu_{i,0}=\frac12,\qquad
 \mu_{i,x}=\frac12-\delta\left(1+\frac{x-1}{K-1}\right),\quad 1\le x<K.
\]
Every arm's mean for the sole player may be $\pi_{x,i}=1/2$. The unique POSM assigns the player to arm $0$; thus $E_i^*=\{0\}$ and $\Delta_{\min}=\delta$. Changing one $\mu_{i,x}$ to $1/2+\varepsilon$ and using \eqref{eq:learning-lower:one-edge} yields
\[
 \liminf_{T\to\infty}\frac{\mathbb E D(T)}{\ln T}
 \ge\sum_{x=1}^{K-1}\frac1{\operatorname{kl}(\mu_{i,x},1/2)}
 \ge\frac{K-1}{16\delta^2}.
\]
The last inequality follows because each deficit $1/2-\mu_{i,x}$ is smaller than $2\delta$.

This family allows a gap interval independent of $K$, while the preceding family isolates arm-side learning. Both comparisons fix the instance before taking the horizon limit; they are not uniform in jointly varying $T,K,\delta$. At every finite horizon, the deterministic bound $D(T)\le T$ still applies.

\subsubsection{Recovery and learning on the same fixed instance}
\label{sec:learning-lower:recovery}

The arm-side family also links learning to recovery. We now impose the model's local information restrictions: arms may retain local state and accepted statistics, but departures are not publicly announced. We adapt the hidden-departure argument from Section~\ref{sec:tradeoff-lower-proof} by coupling the executions until the first static mismatched round after a prescribed departure. Both the statistical argument and the recovery argument will bound the cost on this same static instance. Recall from \eqref{eq:budget-iteration-count} that $N_g(T)=\#\{j:r_j<T\}$, where $r_0=2$ and $r_{j+1}=r_j+g(r_j)$.

\begin{proposition}[A joint obstruction on the arm-side family]
\label{prop:learning-lower:joint}
Let $I_{K,\Delta}$ be the static instance of Section~\ref{sec:learning-lower:arm-side} and let $I_\tau$ delete $p_1$ at the predetermined round $\tau\ge2$. Define the expected post-deletion cost
\[
 L_\Pi(\tau,h)=\mathbb E\left[D_\Pi(\tau+h;I_\tau)-D_\Pi(\tau;I_\tau)\right].
\]
Let $g:\mathbb N_{\ge1}\to\mathbb N_{\ge1}$ be nondecreasing. Suppose the same local protocol is uniformly efficient and satisfies
\[
 L_\Pi(\tau,h)\le Ag(\tau)+C+\eta h\qquad(\tau\ge2,\ h\ge1)
\]
for fixed finite $A,C\ge0$ and $\eta\in(0,1)$. The constants $A$ and $C$ may depend on this fixed family, but not on $\tau$ or $h$. Then, with this instance fixed,
\begin{equation}
 \mathbb E D_\Pi(T;I_{K,\Delta})
 =\Omega_{A,C,\eta}\!\left(N_g(T)+(K-1)\Delta^{-2}\log T\right).
\label{eq:learning-lower:joint}
\end{equation}
The recovery requirement is a separate assumption on the fixed-mean deletion family.
\end{proposition}
\begin{proof}
\emph{Coupling after deletion.} Deleting $p_1$ preserves all other owner pairs and moves $p_0$ to the vacated arm $0$, changing the survivors' POSM. Couple the static and deletion executions using common algorithmic randomness and common rewards on accepted survivor edges. Until the first static mismatched round at or after deletion, each surviving player and its originally assigned arm have identical local states and observations in the two executions. No survivor visits the deleted player's original arm during this coupled prefix, so that arm's changed state cannot convey the deletion elsewhere. The unchanged survivor assignment differs from the new POSM, and every round of the coupled prefix is therefore mismatched in the deletion execution.

\emph{Packing disjoint windows.} Let $d$ be the expected static cost in the augmented interval $\{\tau,\ldots,\tau+h\}$. The probability of any static mismatch there is at most $d$. If none occurs, all $h$ recovery rounds $\tau+1,\ldots,\tau+h$ are mismatched in the deletion execution. Its expected recovery cost is therefore at least $h\max\{0,1-d\}$. The augmented interval includes the deletion round to allow for detection in that round. The recovery condition therefore bounds the static expected cost below by a positive constant whenever $h$ is at least $2(Ag(\tau)+C)/(1-\eta)$. Using $g\ge1$ to absorb $C$ into the coefficient $A+C$, put
\[
          q=\max\{1,\lceil2(A+C)/(1-\eta)\rceil\}.
\]
Set $x_0=2$ and $x_{j+1}=x_j+qg(x_j)+1$. Apply the recovery bound at $\tau_j=x_j$ with $h_j=qg(x_j)$ and charge the disjoint augmented intervals $[x_j,x_{j+1})$. Monotonicity and $g\ge1$ give $x_j\le r_{(q+1)j}$, so the endpoint count in Section~\ref{sec:tradeoff-lower-proof} gives
\[
 \mathbb E D_\Pi(T;I_{K,\Delta})
 \ge\frac{1-\eta}{2}\,\max\{0,N_g(T)/(q+1)-1\}.
\]
\Cref{cor:learning-static-lower} also bounds this same expectation below by $(K-1)\Delta^{-2}\log T/8$ for all sufficiently large $T$. The maximum of two nonnegative quantities is at least half their sum, and $N_g(T)\to\infty$ absorbs the fixed subtraction. This proves \eqref{eq:learning-lower:joint}; the maximum inequality allows the rounds charged by the two arguments to overlap.
\end{proof}

For $g(t)=\Omega(t)$, $N_g(T)=O_g(\log T)$ by Section~\ref{sec:tradeoff-growth-proof}, so for fixed $K,\Delta,g$ the statistical term determines the horizon dependence of \eqref{eq:learning-lower:joint}. More generally, uniform efficiency imposes the following necessary condition on the recovery allowance.

\begin{proposition}[Necessary growth of the recovery allowance]
\label{prop:learning-lower:allowance}
Suppose a local uniformly efficient protocol satisfies the preceding recovery condition on one fixed static/deletion family for which the survivors' POSM changes. Then $N_g(T)=o(T^\alpha)$ for every $\alpha>0$. For a finite nondecreasing integer function $g\ge1$, this count condition is equivalent to
\begin{equation}
                   \liminf_{t\to\infty}\frac{\log g(t)}{\log t}\ge1.
\label{eq:learning-lower:allowance}
\end{equation}
\end{proposition}
\begin{proof}
The packing bound applies to every such fixed family, and uniform efficiency gives the necessary count condition. To establish its equivalence with \eqref{eq:learning-lower:allowance}, put $n=N_g(T)$, with the orbit $r_0=2$, $r_{j+1}=r_j+g(r_j)$. Then $r_n\ge T$ and $r_j<T$ for $j<n$, so
\[
                  T-2\le r_n-2=\sum_{j<n}g(r_j)\le n g(T).
\]
If the count condition holds, then $n\le T^\varepsilon$ eventually for each $\varepsilon>0$, which proves \eqref{eq:learning-lower:allowance}.

Conversely, \eqref{eq:learning-lower:allowance} implies $g(x)\ge x^{1-\varepsilon}$ eventually for each $0<\varepsilon<1$. In a dyadic interval $[2^j,2^{j+1})$, consecutive orbit points are separated by at least $2^{j(1-\varepsilon)}$, so the interval contains at most $1+2^{j\varepsilon}$ points. Summing these bounds gives $N_g(T)=O_\varepsilon(T^\varepsilon)$. For any prescribed $\alpha>0$, choose $\varepsilon<\alpha$.
\end{proof}

Thus a polynomially sublinear allowance \(g(t)=O(t^{1-\varepsilon})\) is incompatible with uniform efficiency under the stated recovery condition on the same fixed family. Uniform efficiency is stronger than vanishing average cost, so the known-preference question in \cref{sec:lower-bounds} remains separate.

Some allowances just below linear growth do satisfy the necessary condition: for example, \(g(t)=\lceil t/\ln(t+2)\rceil\) for \(t\ge1\), satisfies \eqref{eq:learning-lower:allowance} and has \(N_g(T)\sim\tfrac12(\ln T)^2\). Indeed, writing \(y_j=\ln r_j\) gives \(y_{j+1}-y_j\sim1/y_j\), and hence \(y_{j+1}^2-y_j^2\to2\); the stated count follows by summation. A matching learning upper bound would require a further construction.

\subsubsection{The separate cost of the population prefix}
\label{sec:learning-lower:prefix}

To account for the population prefix, consider the following arrival sequence. For an integer $t_*\ge1$, let a new player arrive in every round $1,\ldots,t_*$, replacing its predecessor; the last one remains forever. In this separate construction, each entrant's player means are unknown when its first proposal is chosen. Choose each new player's best arm independently and uniformly in advance by permuting a fixed strictly ordered set of interior Bernoulli means. Before that player's first proposal, no sample from its reward distributions is available. Set, for example,
\[
         \pi_{x,p_r}=\frac14+\frac{r}{2(t_*+1)},\qquad r=1,\ldots,t_*,
\]
at every arm. These means give each arm a strict ranking of players and reveal nothing about the new player's independently chosen permutation.

Even a central controller with all earlier observations chooses the new player's best arm with probability at most $1/K$. With only one player present, that arm is the POSM assignment. Average over the preselected means, then fix a selection whose expected cost is at least this average. This gives a legal oblivious instance with last event at $t_*$ and
\[
                           \mathbb E D(t_*)\ge(1-1/K)t_*.
\]
The case $t_*=1$ is a static instance initialized in round $1$. This construction gives a lower bound on the cost accumulated during the population prefix, on a separate instance family. It does not bound the rate of recovery after an event. Adding this cost to the static statistical lower bound would require a joint construction.

\subsubsection{Interpretation of the comparison}
\label{sec:learning-lower:interpretation}

On the hard family in Section~\ref{sec:learning-lower:arm-side}, the stable matching is unique, so unstable-round loss and POSM-mismatch loss coincide. The information program in Section~\ref{sec:learning-lower:program} extends the comparison to markets with several stable matchings: it charges a stable assignment whenever that assignment is not player-optimal. This distinction accounts for the separation from the binary-stability lower bound of \cite{basu2025super}.

Reward-regret results, such as those for common arm priorities in \cite{SBA21}, measure loss through reward differences, whereas $D(T)$ charges the whole mismatched market once per round. The gap dependence for one loss cannot be transferred directly to the other. For POSM mismatch, the upper bound and the displayed lower-bound families agree in their logarithmic horizon and inverse-square gap orders for fixed $K$. The optimal dependence on the number of arms remains open.
