# Supplementary material for: Decentralized Dynamic Stable Matching
Source: arXiv:2610.41912 source file (2026-11-06)
Supplement: Supplementary file 2 [file accounting.tex]

% \subsection{All-prefix accounting and the main theorem}
% \label{sec:proof-accounting}

% We establish \cref{thm:known} through the following quantitative bound. With the constants in \eqref{eq:parameters} and \eqref{eq:maintenance-window-budget}, for every integer \(K\ge2\), every legal finite-event instance \(I\), and every integer horizon \(T\ge0\), the same protocol satisfies
% \begin{equation}
%   D(T;I)\le
%   \min\!\left\{T,\,
%   32(u+H)+U\left[1+\left\lceil\log_2(T+2)\right\rceil\right]\right\},
%   \qquad T\ge0.
%   \label{eq:all-prefix-bound}
% \end{equation}

% \begin{proof}[Proof of \cref{thm:known}]
% Fix \(I,T\). If the final market is nonempty, \eqref{eq:recovery-time} gives a calibrated handoff at \(V_2\le32(u+H)\). Charge every earlier round at one. Starting with the second mature output at \(m=0\), \cref{lem:maintenance} gives \(L_m\ge2^mH\). A maintenance window beginning at \(Q_m=o_m+L_m<T\) thus has \(2^mH\le Q_m<T\), so at most
% \begin{equation}
%   1+\left\lceil\log_2(T+2)\right\rceil
%   \label{eq:maintenance-window-count}
% \end{equation}
% windows have begun. Each costs at most \(U\), including an unfinished final window. Adding these charges proves \eqref{eq:all-prefix-bound} for \(T\ge V_2\), using also \(D(T;I)\le T\).

% For \(T<V_2\), use \(D(T;I)\le T<V_2\le32(u+H)\). This covers prefixes before the last event: \(u=t_*+1\) still refers to the full instance path. If the final market is empty, no cost occurs after its last event, so \(D(T;I)\le\min\{T,u\}\). Thus \eqref{eq:all-prefix-bound} holds for every \(T\ge0\), including \(T=0\).

% For \(K\ge2\), \(U=2K^2+14K\le9K^2\), and
% \begin{equation}
%   32H+2U=512K^2+72-(K-2)(380K+92)\le512K^2+72.
%   \label{eq:constants-all-prefix}
% \end{equation}
% Using \(1+\lceil\log_2(T+2)\rceil\le2+\ln(T+2)/\ln2\), \(u\ge1\), and \(9/\ln2<13\),
% \[
% \begin{aligned}
%   D(T;I)&\le32u+512K^2+72+\frac9{\ln2}K^2\ln(T+2)\\
%         &\le512(u+K^2)+13K^2\ln(T+2).
% \end{aligned}
% \]
% Since \(\ln(T+2)\ge\ln2\), this is \(O(u+K^2\log(T+2))\) with absolute constants. The protocol and constants are independent of \(I,T\).
% \end{proof}

% For fixed \(K\) and a fixed legal finite-event instance \(I\), \(u<\infty\) is constant, so the all-prefix bound gives \(D(T;I)/T\to0\), even with indefinitely continuing maintenance.
