# Supplementary material for: Decentralized Dynamic Stable Matching
Source: arXiv:2610.41912 source file (2026-11-06)
Supplement: Supplementary file 3 [file general-budgets.tex]

\subsection{Compiling a general recovery scale}
\label{sec:tradeoff-upper-proof}

We construct the replay-length rule in \cref{lem:known-scale-rule}, prove its recovery and iteration bounds, and then record finite-horizon estimates and the post-event recovery guarantee.

\paragraph{Construction of the waiting rule.}
Fix a nondecreasing, polynomial-time computable function \(g:\mathbb N_{\ge1}\to\mathbb N_{\ge1}\) with \(g(t)=\Omega(t)\), and put
\[
 M_g=\max\left\{1,\sup_{t\ge1}\frac{t}{g(t)}\right\}<\infty.
\]
The asymptotic linear lower bound controls the ratios for all sufficiently large \(t\), and positivity controls the remaining finite set. The constant \(M_g\) is used only in the analysis. Define \(F_g:\mathbb N_{\ge1}\to\mathbb N_{\ge1}\) by
\begin{align}
 s_0&=H, &s_{j+1}&=s_j+g(s_j),\nonumber\\
 A_g(x)&=\max\bigl(\{g(s_j)-s_j:64s_j\le x\}\cup\{0\}\bigr),
 &F_g(x)&=H+2x+A_g(x).
 \label{eq:budget-waiting-rule}
\end{align}
The maximum is nonnegative and nondecreasing in \(x\), even though the individual differences need not increase with \(j\). Hence \(F_g\) is nondecreasing and satisfies \eqref{eq:general-wait-condition}.

Since \(s_{j+1}\ge(1+1/M_g)s_j\), evaluation visits \(O_g(1+\log(x+1))\) eligible scales. It calls \(g(s_j)\) only while \(64s_j\le x\), and maintains the maximum of the differences. The assumed polynomial-time computability of \(g\), together with integer additions and comparisons, therefore gives a polynomial-time evaluation of \(F_g\). The protocol \(\Pi_g\) uses \eqref{eq:general-wait-update} with this function, fixed by \(K,g\) before the instance and horizon; it does not need \(M_g\) as an input.

\begin{proof}[Proof of \cref{lem:known-scale-rule}]
The construction above is polynomial-time computable and satisfies the waiting-rule condition. We bound the recovery prefix and then compare the iterates of this rule with those of the given scale.

\paragraph{Bounding the recovery prefix.}
The recovery map is
\[
 \Psi_{F_g}(x)=3x+6H+A_g(x+H).
\]
We show
\begin{equation}
 \Psi_{F_g}^{\circ3}(t+1)\le C_g(t),\qquad
 C_g(t)=
 \begin{cases}
  105H,&1\le t<H,\\
  118(t+g(t)),&t\ge H.
 \end{cases}
 \label{eq:budget-recovery-envelope}
\end{equation}
For an integer \(t\ge H\), choose \(s_j\le t<s_{j+1}\) and put \(a=s_{j+1}\). Then
\[
 t+1\le a=s_j+g(s_j)\le t+g(t),\qquad H\le a.
\]
Whenever \(z+H<64a\), only indices \(k\le j\) can be activated, so \(A_g(z+H)\le\max_{k\le j}s_{k+1}=a\). Writing \(z_0=t+1\) and \(z_{i+1}=\Psi_{F_g}(z_i)\) gives
\[
 \begin{array}{lll}
 z_0+H\le2a,&z_1\le10a,\\
 z_1+H\le11a,&z_2\le37a,\\
 z_2+H\le38a,&z_3\le118a\le118(t+g(t)).
 \end{array}
\]
Every input stays below \(64a\). For \(1\le t<H\), \(z_0\le H\), and the three inputs to \(A_g\) are at most \(2H,10H,34H\), below the first threshold \(64H\). Thus all three additional terms vanish and
\[
 z_3=27(t+1)+78H\le105H.
\]
This proves \eqref{eq:budget-recovery-envelope} without any bound on \(g(t+1)/g(t)\). The function \(C_g\) is nondecreasing, including at \(H\).

\paragraph{Counting maintenance windows.}
Let \(b_0=H\) and \(b_{j+1}=F_g(b_j)\). Since \(F_g(x)\ge2x\), six iterations from \(s_j\) reach at least \(64s_j\), and
\[
 F_g(64s_j)\ge H+128s_j+g(s_j)-s_j
             \ge s_j+g(s_j)=s_{j+1}.
\]
Monotonicity therefore gives
\[
 b_{7j}\ge s_j,\qquad
 N_{F_g}(T)\le7\#\{j:s_j<T\}\le7N_g(T).
\]
Indeed, if \(m=\#\{j:s_j<T\}\), then \(b_{7m}\ge s_m\ge T\); also \(r_0=2\le H=s_0\) and monotonicity imply \(r_j\le s_j\). These comparisons include horizons equal to an iterate.

Since \(t\le M_g g(t)\) and \(H\le16K^2\), \eqref{eq:budget-recovery-envelope} gives the first bound in \cref{lem:known-scale-rule}, with a constant depending only on \(g\). The identity \(b_j=F_g^{\circ j}(H)\) gives the second with the universal constant \(7\). When \(g(t)=t\), every difference in \(A_g\) vanishes, so \(F_g(x)=H+2x\) for all \(x\ge1\).
\end{proof}

\paragraph{Finite-horizon estimates.}
Combining the two bounds above with \cref{lem:general-wait-interface} gives
\begin{equation}
 D_{\Pi_g}(T;I)
 \le\min\{T,118(t_*+g(t_*))+105H+7U N_g(T)\}.
 \label{eq:budget-finite-dynamic}
\end{equation}
For a static instance, \(t_*=1<H\), so the stronger bound is
\begin{equation}
 \sup_{I:\,t_*=1}D_{\Pi_g}(T;I)\le105H+7U N_g(T).
 \label{eq:budget-finite-static}
\end{equation}
Since \(H\le16K^2\), \(U\le9K^2\), and \(t_*\le M_g g(t_*)\), the dynamic estimate is \(O_g(g(t_*)+K^2[1+N_g(T)])\), with a constant independent of \(K,I,T\). The static estimate has constants uniform in \(K,g,I,T\). All shorter prefixes, including \(T=0\), and the empty-market case are covered by the interface. The proof of \cref{thm:general-budget-upper} in \cref{sec:known-analysis} absorbs the startup term and handles the small horizons.

\begin{proof}[Proof of \cref{cor:flexible-sublinear}]
We first bound the cost after calibration, then include the recovery prefix and choose the accuracy coefficients.

\paragraph{Cost after calibration.}
We verify the window guarantee used in \cref{sec:tradeoff-problem} directly from the actual maintenance windows. Fix \(\eta\in(0,1)\). The interface recurrences give
\[
 L_j\ge(2^{j+1}-1)H,\qquad
 Q_{j+1}-Q_j=c_j+L_{j+1}\ge(2^{j+2}-1)H.
\]
Every \([Q_j,V_{j+1})\) costs at most \(U\), and \(Q_0>V_{\mathrm{cal}}\). Put
\[
 m_\eta=\min\{m\in\mathbb Z_{\ge0}:(2^{m+2}-1)H\ge U/\eta\},\qquad
 Q_{K,\eta}=(m_\eta+1)U.
\]
Charge the first \(m_\eta\) windows separately. Later starts are at least \(U/\eta\) apart, so at most \(1+\eta h/U\) occur in any \(h\) consecutive rounds. In particular,
\begin{equation}
 D_{\Pi_g}(V_{\mathrm{cal}}+h;I)-D_{\Pi_g}(V_{\mathrm{cal}};I)
 \le Q_{K,\eta}+\eta h \qquad(h\ge0).
 \label{eq:budget-tail-discount}
\end{equation}
This difference counts rounds \(V_{\mathrm{cal}}+1,\ldots,V_{\mathrm{cal}}+h\). Because \(U/H\le1\), \(Q_{K,\eta}=O(K^2[1+\log(1/\eta)])\), independently of \(g\).

\paragraph{The post-event recovery window.}
Let \(\tau=t_*\) and \(a=V_{\mathrm{cal}}-\tau\) in a nonempty final market. The first \(a\) rounds of the event-excluding window cost at most \(a\le C_g(\tau)\). Splitting a longer window at \(V_{\mathrm{cal}}\) and using \eqref{eq:budget-tail-discount} gives, for every \(h\ge1\),
\begin{equation}
 L_{\Pi_g}(h;I)
 \le \min\{h,C_g(t_*)+Q_{K,\eta}+\eta h\}.
 \label{eq:budget-finite-recovery}
\end{equation}
Empty final markets have zero post-event cost.

\paragraph{Recovery coefficients.}
For \(0<\varepsilon<1\), take \(\eta=\varepsilon/2\) and
\[
 c_\varepsilon=
 \frac{2(118(1+M_g)+105H+Q_{K,\varepsilon/2})}{\varepsilon}>0.
\]
Since \(g(t_*)\ge1\) and \(C_g(t_*)\le118(1+M_g)g(t_*)+105H\), the condition \(h\ge c_\varepsilon g(t_*)\) implies \(L_{\Pi_g}(h;I)\le\varepsilon h\). For \(\varepsilon\ge1\), the claim follows from \(L_{\Pi_g}(h;I)\le h\). Thus the same \(\Pi_g\) has sublinear mismatch cost relative to \(g\); its rule has no accuracy parameter. In particular, the positive coefficient
\begin{equation}
 c^{\star}_{K,g}=4(118(1+M_g)+105H+Q_{K,1/4})=O_g(K^2)
 \label{eq:common-half-recovery}
\end{equation}
is valid uniformly over instances for each fixed \(K,g\). This is the threshold used for the common-coefficient class in \cref{cor:uniform-minimax-maintenance}.
\end{proof}

\paragraph{Comparison of integer scales.}
The growth examples in the next section use integer representatives of the displayed real-valued shapes. The following comparison shows that representatives within constant factors have the same iteration-count order. For nondecreasing positive integer scales \(g\le\widetilde g\le c g\) with \(g(t)=\Omega(t)\), put
\[
 Q_g(x)=x+g(x),\qquad
 d=\max\{1,\lceil c\rceil\}.
\]
Monotonicity gives \(Q_g^{\circ d}(x)\ge x+d g(x)\ge x+\widetilde g(x)\), and hence
\[
 Q_g(x)\le Q_{\widetilde g}(x)\le Q_g^{\circ d}(x).
\]
Iterating from \(2\) gives \(N_{\widetilde g}(T)\le N_g(T)\le dN_{\widetilde g}(T)\). For two nondecreasing positive integer scales with at least linear asymptotic growth and within constant factors, apply this comparison to their pointwise minimum and maximum. Thus their iteration counts have the same order even when neither scale dominates the other everywhere. The comparison is a growth statement; computational admissibility is the separate hypothesis in \cref{thm:general-budget-upper}, verified for the integer representatives in \cref{sec:tradeoff-growth-proof}.
