# Supplementary material for: Decentralized Dynamic Stable Matching
Source: arXiv:2610.41912 source file (2026-11-06)
Supplement: Supplementary file 4 [file known-preferences.tex]

% !TeX root = ../main.tex
\section{Details for Tracking with Known Preferences}
\label{app:known-proofs}
\label{sec:proof}
This appendix gives the local state definitions and the coordination arguments underlying \cref{lem:known-recovery,lem:known-maintenance}. Their proofs appear in \cref{sec:proof-recovery,sec:proof-maintenance}; \cref{sec:tradeoff-upper-proof} proves the replay-rule construction in \cref{lem:known-scale-rule}. The resulting proofs of \cref{thm:general-budget-upper,thm:known} are in \cref{sec:known-analysis}.

For the analysis, permit any nondecreasing computable waiting rule \(F:\mathbb N_{\ge1}\to\mathbb N_{\ge1}\) satisfying
\begin{equation}
 F(x)\ge H+2x.
 \label{eq:general-wait-condition}
\end{equation}
Keep every control rule of Algorithm~\ref{alg:scda-core}, replacing only the output update by
\begin{equation}
 y\leftarrow\text{the arm just proposed to},\qquad
 L\leftarrow F(a-\ell),\quad q\leftarrow a+L,\quad \ell\leftarrow a.
 \label{eq:general-wait-update}
\end{equation}
Every actual output uses the old \(\ell\), including an incorrect output or a rejected final proposal. Initialization and the order of all round-start and feedback updates are unchanged. The original algorithm uses \(F(x)=H+2x\). The lemmas below apply to the general rule.

\input{appendices/tradeoffs/local-protocol}
\input{appendices/tradeoffs/mature-executions}
\input{appendices/tradeoffs/sweep-isolation}
\input{appendices/tradeoffs/recovery}
\input{appendices/tradeoffs/maintenance}
\input{appendices/tradeoffs/accounting}
