# Supplementary material for: Decentralized Dynamic Stable Matching
Source: arXiv:2610.41912 source file (2026-11-06)
Supplement: Supplementary file 5 [file local-protocol.tex]

\subsection{Local state, auxiliary operations, and round order}
\label{sec:local}

We give the state definitions, equivalent auxiliary operations, and round order used to analyze \cref{alg:scda-core}, including histories that do not satisfy the mature-entry conditions. In \cref{eq:sweep}, \(\sigma_{2j-1}=0,\ \sigma_{2j}=j\) for \(1\le j\le K-1\), and the last two entries are zero.

The persistent state of player \(i\) consists of its ranking and \(a,y,\ell,\rho\). Here \(\rho\) is the length of the current consecutive suffix of actual accepted BUS proposals, capped at \(J\), and is updated in every mode. At birth,
\begin{equation}
  a=\ell=\rho=0,\qquad y=p_i(1),\qquad m=\SEEK .
  \label{eq:initialization}
\end{equation}
The temporary state consists of the mode \(m\), a scheduled next-round mode \(\nu\), a flag \(\mathit{seenR}\) recording whether this visit to \(\SEEK\) has seen a BUS rejection, a scan position \(s\) and block-success flag \(\mathit{blockOK}\), work counters \(h,k\), and the replay deadline \(q\). At a work action, \(h=0,\ldots,J-1\) counts completed rounds of that invocation, so the current action is work round \(h+1\).

\paragraph{Mode entry.}
The operation \(\operatorname{Enter}(m')\) first saves the requested mode \(m'\), then sets \(m\gets m'\) and \(\nu\gets\none\), clears the old mode-specific state, and leaves \(a,y,\ell,\rho\) unchanged. Thus a call \(\operatorname{Enter}(\nu)\) uses the pending mode before clearing it. It initializes the new mode as follows:
\[
\begin{array}{c|l}
  m' & \text{new mode-specific state}\\ \hline
  \SEEK   & \mathit{seenR}\gets\false\\
  \SWEEP  & s\gets 1,\quad \mathit{blockOK}\gets\true\\
  \WORK   & h\gets 0,\quad k\gets 1\\
  \REPLAY & \text{retain the deadline }q\text{ just computed at output}.
\end{array}
\]
Only a real work output updates \(\ell\). In particular, returning to \(\SEEK\) discards the old rejection flag but preserves the continuous BUS counter \(\rho\). Entering \(\REPLAY\) discards the other temporary state while retaining \(q\).

\paragraph{Proposal and feedback.}
The operation \(\operatorname{Pull}(x)\) makes one real proposal to arm \(x\), observes \(z\in\{\A,\R\}\) and the utility if accepted, updates
\[
  \rho\gets
  \begin{cases}
    \min\{J,\rho+1\},&x=\BUS\text{ and }z=\A,\\
    0,&\text{otherwise},
  \end{cases}
\]
and returns \(z\). This update applies in every mode and precedes the mode-specific feedback rules, so the AA handoff uses the updated value of \(\rho\).

\paragraph{Sweep advancement.}
The operation \(\operatorname{AdvanceSweep}(z)\) is called only in \(\SWEEP\) after a BUS rejection has been ruled out. It first sets \(\mathit{blockOK}\gets\mathit{blockOK}\wedge(z=\A)\), then applies exactly one of the following updates:
\begin{enumerate}[label=(\roman*)]
  \item If \(s<2K\), set \(s\gets s+1\).
  \item If \(s=2K\) and \(\mathit{blockOK}=\true\), set \(\nu\gets\WORK\).
  \item If \(s=2K\) and \(\mathit{blockOK}=\false\), set \(s\gets1\) and \(\mathit{blockOK}\gets\true\).
\end{enumerate}
A non-BUS rejection therefore marks the block as failed without rewinding its position. A failed block restarts at its first action in the next round. On a BUS rejection, the main controller instead sets \(\nu\gets\SEEK\) and skips this operation, including at \(s=2K\); this branch takes priority over the block-completion test.

\paragraph{Work action.}
The local action-selection function is
\[
  \operatorname{WorkArm}_i(h,k)=
  \begin{cases}
    \PARK,&0\le h<2K,\\
    p_i(1),&2K\le h\le4K,\\
    p_i(k),&4K<h<J.
  \end{cases}
\]
These are the \phase{Park}, \phase{Top}, and \phase{DA} portions of \(\WORK\). The main controller advances \(k\) only after a rejection in a nonfinal \phase{DA} round. In the final round it saves the actual proposed arm regardless of feedback and computes \(L\) using the old \(\ell\) before assigning \(\ell\gets a\), exactly as in \cref{eq:output}.

At every actual output, \(a-\ell\ge1\): the first output has \(\ell=0\) and \(a\ge J-1>0\), and subsequent outputs occur in strictly later local rounds than the output recorded in \(\ell\).

\paragraph{Round order.}
At each round's start, the environment applies entries and exits. This is not an event notification available to the player. Each present player then executes its previously scheduled mode change, checks replay expiration, and checks scan qualification, in that order. Scan qualification is checked only in \(\SEEK\), so it neither interrupts \(\WORK\) nor extends \(\REPLAY\). The player makes exactly one proposal, updates \(\rho\), handles feedback in the current mode, and increments \(a\).

Each loop iteration contains exactly one call to \(\operatorname{Pull}\). The operations \(\operatorname{Enter}\), \(\operatorname{AdvanceSweep}\), and \(\operatorname{WorkArm}_i\) are local state operations and consume no additional rounds.

Feedback-triggered mode changes take effect in the next round. Expiration and qualification checks affect the current round's action. A scheduled \(\WORK\) is therefore a pending transition, not an extra phase with its own actions. It arises only from a qualified AA pair in \(\SEEK\) or a successful complete scan.
