# Supplementary material for: Decentralized Dynamic Stable Matching
Source: arXiv:2610.41912 source file (2026-11-06)
Supplement: Supplementary file 6 [file maintenance.tex]

\subsection{Calibration and bounded maintenance}
\label{sec:proof-maintenance}

\paragraph{Calibration from actual consecutive outputs.}
Consider two mature executions in a fixed market of \(1\le n\le K\) players, consecutive in every player's actual output sequence. Label players by decreasing BUS preference, write \(m^*\) for the POSM, and let \(o_{m-1},o_m\) be the root's output times.

By \cref{lem:mature}, player \(j\), born at \(b_j\), outputs at local ages \(a_{j,r}=o_r+2(j-1)-b_j\) for \(r=m-1,m\). Actual adjacency gives the old register \(\ell_j=a_{j,m-1}\), so the update uses
\[
  a_{j,m}-\ell_j=o_m-o_{m-1},\qquad
  L_m=F(o_m-o_{m-1}).
\]
Thus the replay lengths agree, while the global deadlines retain the output offsets:
\begin{equation}
  Q_{j,m}=o_m+2(j-1)+L_m.
  \label{eq:common-wait-deadlines}
\end{equation}

\begin{sublemma}[Bounded maintenance under a general waiting rule]
\label{lem:maintenance}
Suppose two mature executions in a fixed nonempty market give consecutive actual outputs for every player, and the population remains fixed thereafter. Every subsequent maintenance cycle produces each player's next actual output in a mature execution, preserving the output offsets and a common waiting length. For cycle \(m\), let \(o=o_m\) and \(L=L_m\) be the current root output time and common waiting length, and put \(Q=o+L\). If \(o'\) is the next root output and \(V'\) its handoff completion round, then
\[
  0<C_m:=o'-Q\le2J+2K-1,\qquad
  V'-Q\le U=2K^2+14K,
\]
and
\[
  L_{\mathrm{next}}=F(L+C_m)\ge H+2(L+C_m)>2L.
\]
The maintenance window is \([Q,V')\); between these windows, \(M_t=m^*\).
\end{sublemma}

\begin{proof}[Proof of \cref{lem:maintenance,lem:known-maintenance}]
We induct on calibrated handoffs. The deadlines are \(Q+2(j-1)\) by \eqref{eq:common-wait-deadlines}, and \(L\ge H>2K\) places \(Q\) after the current handoff. Correct replay lasts until \(Q\); every other current replay ends by \(Q+2K-2\), possibly earlier after rejection. Once the root scans, \cref{lem:sweep}(i) excludes other work, scans, and outputs.

\emph{If \(m^*(1)\ne\BUS\)}, the root enters fresh \SEEK{} at \(Q\) with \(\rho=0\) and its rejection record cleared. Its \(J\) BUS acceptances in \(Q,\ldots,Q+J-1\) cannot trigger its own AA handoff and prevent every other AA start. Any other BUS replayer is rejected at \(Q\), before its own deadline, resetting its counter; non-BUS replayers already have zero counters. Thus no competing scan or work begins. Since \(J>2K-2\), all others are seekers when the root starts scanning at \(Q+J\), and the first block succeeds:
\begin{equation}
  c=Q+J+2K.
  \label{eq:maintenance-nonbus-entry}
\end{equation}

\emph{If \(m^*(1)=\BUS\)}, all \(L\ge H>J\) proposals in \(o,\ldots,Q-1\), including the output round \(o\), are accepted at BUS. The counter is saturated, so expiration followed by qualification starts \SWEEP{} at \(Q\). All other replays end by \(Q+2K-2\), so the second block, starting at \(Q+2K\), succeeds unless the first already did. Hence
\begin{equation}
  c\le Q+4K\le Q+J+2K.
  \label{eq:maintenance-bus-entry}
\end{equation}

In both cases, no output occurs between the current handoff and \(c\), and \(c\le Q+J+2K\). By \cref{lem:sweep}(ii) and \cref{lem:mature}, the next execution is mature and gives each player's next actual output with the same offsets. Since \(o'=c+J-1\),
\begin{equation}
  C_m:=o'-Q,\qquad 0<C_m\le2J+2K-1.
  \label{eq:maintenance-overhead}
\end{equation}
Calibration therefore applies again with \(o'-o=L+C_m\):
\begin{equation}
  L_{\mathrm{next}}=F(L+C_m)\ge H+2(L+C_m)>2L.
  \label{eq:wait-doubling}
\end{equation}

The last player enters \REPLAY{} one round after its output, so \(V'=o'+2(n-1)+1\le o'+2K-1\), giving
\begin{equation}
  V'-Q\le C_m+2K-1\le2J+4K-2=2K^2+14K=U.
  \label{eq:maintenance-window-budget}
\end{equation}
Thus \([Q,V')\) costs at most \(U\) mismatch rounds. Since \(L_{\mathrm{next}}\ge H>2K\), the next deadline follows \(V'\), with correct replay between the windows, completing the induction. Finally, \(L_0\ge H\), and monotonicity gives \(L_{\mathrm{next}}=F(L+C_m)\ge F(L)\). Applied to the pair supplied by \cref{lem:recovery}, these bounds prove \cref{lem:known-maintenance}.
\end{proof}


% \subsection{Calibration and bounded maintenance}
% \label{sec:proof-maintenance}

% \paragraph{Calibration from actual consecutive outputs.}
% Consider two mature executions in the same fixed market, consecutive in every player's actual output sequence. Label players by decreasing BUS preference, write \(m^*\) for the POSM, and let \(o_{m-1},o_m\) be the root's output times.

% \begin{proof}[Proof of the calibration identity]
% By \cref{lem:mature}, player \(j\), born at \(b_j\), outputs at local ages \(a_{j,r}=o_r+2(j-1)-b_j\) for \(r=m-1,m\). Actual adjacency, obtained initially from \cref{lem:recovery}, gives the old register \(\ell_j=a_{j,m-1}\). Before this register is overwritten, the local update satisfies
% \[
%   a_{j,m}-\ell_j=o_m-o_{m-1},\qquad
%   L_m=F(o_m-o_{m-1}).
% \]
% This common length gives global deadlines
% \begin{equation}
%   Q_{j,m}=o_m+2(j-1)+L_m,
%   \label{eq:common-wait-deadlines}
% \end{equation}
% preserving the output offsets.
% \end{proof}

% \begin{sublemma}[Bounded maintenance under a general waiting rule]
% \label{lem:maintenance}
% Suppose two actual consecutive mature executions occur in the same fixed nonempty market, and the population remains fixed thereafter. Every subsequent maintenance cycle produces each player's next actual output in a mature execution, preserving the fixed output offsets and a common waiting length. Let \(o\) and \(L\) be the current root output time and common waiting length, and let \(Q=o+L\). If \(o'\) is the next root output and \(V'\) the completion round of its handoff, then
% \[
%   0<C_m:=o'-Q\le2J+2K-1,\qquad
%   V'-Q\le U=2K^2+14K,
% \]
% and
% \[
%   L_{\mathrm{next}}=F(L+C_m)\ge H+2(L+C_m)>2L.
% \]
% The maintenance window is \([Q,V')\); between these windows, \(M_t=m^*\).
% \end{sublemma}

% \begin{proof}[Proof of \cref{lem:maintenance,lem:known-maintenance}]
% The computations supplied by \cref{lem:known-recovery} are mature, as established in \cref{sec:proof-recovery}, so it suffices to prove the stronger statement above. We induct on calibrated handoffs. The deadlines are \(Q+2(j-1)\) by \eqref{eq:common-wait-deadlines}, and \(L\ge H>2K\) places \(Q\) after the current handoff. Correct replay lasts until the root returns at \(Q\); each other current replay ends by \(Q+2K-2\), possibly earlier after rejection. Once the root scans, \cref{lem:sweep}(i) excludes other work, scans, and outputs.

% \emph{If \(m^*(1)\ne\BUS\)}, the root has \(\rho=0\) at \(Q\) and enters fresh \SEEK{} with its rejection record cleared. Its \(J\) BUS acceptances in \(Q,\ldots,Q+J-1\) cannot trigger its own AA handoff and prevent every other AA start. Any other BUS replayer is rejected at \(Q\), before its own deadline, resetting its counter; non-BUS replayers already have zero counters. Thus no competing scan or work begins. Since \(J>2K-2\), all other players are seekers when the root starts scanning at \(Q+J\), and the first block succeeds. Hence
% \begin{equation}
%   c=Q+J+2K.
%   \label{eq:maintenance-nonbus-entry}
% \end{equation}

% \emph{If \(m^*(1)=\BUS\)}, the \(L\ge H>J\) proposals in \(o,\ldots,Q-1\), including the output round \(o\), are accepted at BUS. The counter is saturated, so expiration followed by qualification starts \SWEEP{} in the same round \(Q\). All other replays end by \(Q+2K-2\), so the second block, starting at \(Q+2K\), succeeds unless the first already did. Thus
% \begin{equation}
%   c\le Q+4K\le Q+J+2K.
%   \label{eq:maintenance-bus-entry}
% \end{equation}

% Neither case permits an output between the current handoff and \(c\). The next execution is mature by \cref{lem:sweep}(ii), and \cref{lem:mature} gives each player's next actual output, with the same offsets. Since \(o'=c+J-1\),
% \begin{equation}
%   C_m:=o'-Q,\qquad 0<C_m\le2J+2K-1=:\overline C.
%   \label{eq:maintenance-overhead}
% \end{equation}
% The two outputs are actually adjacent, so calibration applies again with \(o'-o=L+C_m\):
% \begin{equation}
%   L_{\mathrm{next}}=F(L+C_m)\ge H+2(L+C_m)>2L.
%   \label{eq:wait-doubling}
% \end{equation}

% Finally, \(V'=o'+2(n-1)+1\le o'+2K-1\), giving
% \begin{equation}
%   V'-Q\le C_m+2K-1\le2J+4K-2=2K^2+14K=U.
%   \label{eq:maintenance-window-budget}
% \end{equation}
% Each physical round costs at most one in \(D\), so \([Q,V')\) costs at most \(U\). Since \(L_{\mathrm{next}}\ge H>2K\), the next deadline follows \(V'\), with correct replay between the windows. This preserves the induction. Finally, \(L_0\ge H\) follows from the waiting-rule condition, and monotonicity gives \(L_{\mathrm{next}}=F(L+C_m)\ge F(L)\); together with the uniform bound \(U=O(K^2)\), these are the claims of \cref{lem:known-maintenance}.
% \end{proof}
