# Supplementary material for: Decentralized Dynamic Stable Matching
Source: arXiv:2610.41912 source file (2026-11-06)
Supplement: Supplementary file 8 [file recovery.tex]

\subsection{Recovery to consecutive mature executions}
\label{sec:proof-recovery}

The waiting rule \(F\) satisfies \eqref{eq:general-wait-condition}. Define the nondecreasing recovery map
\begin{equation}
 \Psi_F(x)=x+F(x+H)+3H.
 \label{eq:general-recovery-map}
\end{equation}

\begin{sublemma}[Recovery to actual consecutive mature outputs]
\label{lem:recovery}
For every normally initialized finite-event history with a nonempty final market, two mature handoffs beginning after \(t_*\) complete by a round
\begin{equation}
 V_{\mathrm{cal}}\le\Psi_F^{\circ3}(t_*+1).
 \label{eq:recovery-time}
\end{equation}
Each player's two outputs are consecutive in its actual output history, so the second output uses the local age of the first as its old \(\ell\).
\end{sublemma}

\begin{proof}[Proof of \cref{lem:recovery,lem:known-recovery}]
Let \(n\) be the final population size and \(z\) its highest-priority player at BUS. States are taken after round-start updates. At any output in round \(v\), including an incorrect one, a player born at \(b_i\ge1\) has \(0\le\ell\le a=v-b_i\le v\). By monotonicity of \(F\), the old register \(\ell\) gives the global deadline
\begin{equation}
 Q_i=v+F(a-\ell)\le v+F(v).
 \label{eq:replay-deadline-bound}
\end{equation}
Replay expires in its deadline round; acceptance never extends it, and rejection can end it earlier.

\paragraph{First mature handoff.}
From round \(t_*+1\), \(z\) is never rejected at BUS. Before reaching a continuing scan, it can produce at most one output from inherited work or an old seek rejection record, and any such output occurs by \(t_*+J+2\). A fresh seek clears that record and cannot trigger an AA handoff. By \eqref{eq:replay-deadline-bound}, every preceding replay ends by \(t_*+J+2+F(t_*+J+2)\). At most \(J\) further qualification rounds therefore give a continuing scan by
\begin{equation}
 \beta\le t_*+J+2+F(t_*+J+2)+J
 \le\Psi_F(t_*+1).
 \label{eq:continuing-scan-time}
\end{equation}
An inherited scan already satisfies the isolation invariant from its original qualified entry, even if events occurred in the meantime.

Until success, \cref{lem:sweep}(i) excludes other work, scans, and outputs. All remaining replays therefore expire by \(\beta+F(\beta)\). A residual block and one full block take at most \(4K\) further rounds; the full block succeeds if no earlier one does. By \cref{lem:sweep,lem:mature}, the resulting mature handoff completes at
\begin{equation}
 V_{\mathrm{first}}
 \le\beta+F(\beta)+J+6K-2\le\Psi_F(\beta).
 \label{eq:first-recovery-handoff}
\end{equation}
All players are then in correct \REPLAY{}, although their waiting lengths can differ.

\paragraph{The next work start is mature.}
Before any new work starts, no output replaces the current deadlines, all of which are at most \(V_{\mathrm{first}}+F(V_{\mathrm{first}})\). If no work has started by that round, all current replays have ended. Player \(z\) is then already scanning or qualifies within \(J\) rounds, and a residual block followed by a full block succeeds within at most \(4K\) more rounds. Thus a new work start exists by \(V_{\mathrm{first}}+F(V_{\mathrm{first}})+J+4K\); let \(r\) be the first such start.

Suppose player \(i\) starts through an AA handoff. Its current seek visit began after \(V_{\mathrm{first}}\) with the rejection flag cleared. The final acceptance run must have length exactly two, or work would have started earlier. Hence, in that same visit, \(i\) was rejected at \(r-3\) and accepted at \(r-2,r-1\).

Let \(w\) be the BUS winner at \(r-3\). It outranks \(i\) and remains present, so it must avoid BUS in both following rounds. A winning seeker continues on BUS, including upon scan qualification; a player accepted while replaying BUS proposes there again, including after expiration; and a continuing scan leaves BUS only for isolated rounds. A work entry in either intervening round would contradict the choice of \(r\). This two-round absence is impossible, so the first new work follows a successful scan and is mature by \cref{lem:sweep}(ii).

\paragraph{Consecutive outputs and calibration.}
By \cref{lem:mature}, each player outputs exactly once in each mature execution. No output occurs between the first handoff and \(r\), so these are consecutive actual outputs. The bound on \(r\), followed by \(J+2(n-1)\) handoff rounds, gives
\begin{equation}
 \begin{aligned}
 V_{\mathrm{cal}}
 &\le V_{\mathrm{first}}+F(V_{\mathrm{first}})+2J+6K-2\\
 &\le\Psi_F(V_{\mathrm{first}})
 \le\Psi_F^{\circ3}(t_*+1).
 \end{aligned}
 \label{eq:second-recovery-handoff}
\end{equation}
For \(K\ge2\), \(J+1<H\), \(J+6K-2<H\), and \(2J+6K-2<H\); these inequalities and monotonicity justify all three applications of \(\Psi_F\).

The two mature executions have the same player offsets. Their actual adjacency therefore makes every player's output-age difference equal to the root's inter-output duration. Applying \(F\) gives a common replay length at the second handoff, with staggered deadlines as detailed in \cref{sec:proof-maintenance}. Together with matching correctness, this proves \cref{lem:known-recovery}.
\end{proof}


% \subsection{Recovery to consecutive mature executions}
% \label{sec:proof-recovery}

% The waiting rule \(F\) satisfies \eqref{eq:general-wait-condition}. Define the nondecreasing recovery map
% \begin{equation}
%  \Psi_F(x)=x+F(x+H)+3H.
%  \label{eq:general-recovery-map}
% \end{equation}

% \begin{sublemma}[Recovery to actual consecutive mature outputs]
% \label{lem:recovery}
% For every normally initialized finite-event history with a nonempty final market, two mature handoffs beginning after \(t_*\) complete by a round
% \begin{equation}
%  V_{\mathrm{cal}}\le\Psi_F^{\circ3}(t_*+1).
%  \label{eq:recovery-time}
% \end{equation}
% Their outputs are consecutive in each player's actual output history. Thus, immediately before its second output updates \(\ell\), the register still holds the local age of its first output.
% \end{sublemma}

% \begin{proof}[Proof of \cref{lem:recovery,lem:known-recovery}]
% Let \(n\) be the final population size and \(z\) its highest-priority player at BUS. All states are taken after round-start updates. At an actual output in global round \(v\), a player born at \(b_i\ge1\) has \(0\le\ell\le a=v-b_i\le v\). Monotonicity gives
% \begin{equation}
%  Q_i=v+F(a-\ell)\le v+F(v).
%  \label{eq:replay-deadline-bound}
% \end{equation}
% This bound includes incorrect outputs. Expiration acts in the deadline round; acceptance does not extend the deadline, and rejection can end replay earlier.

% \paragraph{First mature handoff.}
% From round \(t_*+1\), player \(z\) is never rejected at BUS. An inherited work invocation or a seeker with an old rejection record produces at most one output before a fresh seek, by \(t_*+J+2\). A fresh seek clears that record. An inherited replay comes from an earlier output; an inherited scan may continue. Once replay ends, at most \(J\) BUS acceptances give scan qualification. Thus \(z\) reaches a continuing qualified scan by
% \begin{equation}
%  \beta\le t_*+J+2+F(t_*+J+2)+J
%  \le\Psi_F(t_*+1).
%  \label{eq:continuing-scan-time}
% \end{equation}
% An inherited scan retains the isolation invariant from its original qualified entry, even if events occurred in the meantime.

% Until the scan succeeds, \cref{lem:sweep}(i) excludes other work, scans, and outputs. Every remaining replay therefore comes from an output before \(\beta\), and expires by \(\beta+F(\beta)\). Unless success occurs sooner, a residual block and one full block take at most \(4K\) further rounds. The full block succeeds and \cref{lem:sweep,lem:mature} give a mature handoff at
% \begin{equation}
%  V_{\mathrm{first}}
%  \le\beta+F(\beta)+J+6K-2\le\Psi_F(\beta).
%  \label{eq:first-recovery-handoff}
% \end{equation}
% All players are then in correct \REPLAY{}, although their waiting lengths can differ.

% \paragraph{Actual adjacency of the outputs.}
% Consider the first actual work start \(r>V_{\mathrm{first}}\), whose existence is established below. If player \(i\) starts through an AA handoff, its current seek visit began after \(V_{\mathrm{first}}\) with the rejection flag cleared. The acceptances in rounds \(r-2,r-1\) therefore require a rejection at \(r-3\): an acceptance there would either leave the flag clear or have triggered an earlier work start.

% Let \(w\) be the BUS winner at \(r-3\). It outranks \(i\) and remains present, so it must avoid BUS in both \(r-2\) and \(r-1\). No player is in work between the first handoff and \(r\). A winning seeker continues on BUS, including when it qualifies to scan. A player accepted while replaying BUS proposes there again next round, including after expiration. A continuing scan leaves BUS only for isolated rounds. A scheduled work entry in either intervening round would contradict the minimality of \(r\). The required two-round absence is therefore impossible.

% Consequently the first new work follows a successful scan and is mature. \Cref{lem:mature} excludes extra outputs between a player's first mature output and the first handoff; there is no output before the next work starts; and that mature execution gives exactly one new output per player. The two outputs are actual neighbors in each player's history.

% \paragraph{Time of the second handoff.}
% Until that next work starts, no output replaces the deadlines, which are all at most \(V_{\mathrm{first}}+F(V_{\mathrm{first}})\). Once these deadlines expire, \(J\) qualification rounds, at most \(4K\) scan rounds, and \(J+2(n-1)\) handoff rounds suffice. Thus the first new work does exist, and this very next mature handoff satisfies
% \begin{equation}
%  \begin{aligned}
%  V_{\mathrm{cal}}
%  &\le V_{\mathrm{first}}+F(V_{\mathrm{first}})+2J+6K-2\\
%  &\le\Psi_F(V_{\mathrm{first}})
%  \le\Psi_F^{\circ3}(t_*+1).
%  \end{aligned}
%  \label{eq:second-recovery-handoff}
% \end{equation}
% For \(K\ge2\), \(J+1<H\), \(J+6K-2<H\), and \(2J+6K-2<H\); these inequalities and monotonicity justify the three recovery steps. No free reset or arbitrary-state initialization is used.

% Both computations are mature, so \cref{lem:mature} gives correct outputs with the same player offsets. Actual adjacency makes the difference between each player's current output age and its old \(\ell\) equal to the root's inter-output duration. Applying \(F\) therefore gives a common replay length at the second handoff, while the deadlines retain the output offsets, as detailed in \cref{sec:proof-maintenance}. This proves \cref{lem:known-recovery}.
% \end{proof}
