# Supplementary material for: Decentralized Dynamic Stable Matching
Source: arXiv:2610.41912 source file (2026-11-06)
Supplement: Supplementary file 9 [file scda-interface.tex]

\subsection{SC-DA with a general local waiting rule}
\label{sec:tradeoff-native-interface}

The upper bound uses the recovery and maintenance lemmas through the following accounting statement. It bounds the total cost by the calibration prefix and the number of maintenance windows.

Use \(J,H\) from \eqref{eq:parameters} and \(U=2K^2+14K\) from \eqref{eq:maintenance-window-budget}. Fix a nondecreasing computable \(F:\mathbb N_{\ge1}\to\mathbb N_{\ge1}\) satisfying \eqref{eq:general-wait-condition}, and use the update \eqref{eq:general-wait-update}. Define
\[
 b_0=H,\qquad b_{j+1}=F(b_j),\qquad
 N_F(T)=\#\{j\ge0:b_j<T\}.
\]
This auxiliary count is distinct from the budget count \(N_g\).

\begin{sublemma}[Recovery and maintenance under a local waiting rule]
\label{lem:general-wait-interface}
For every normally initialized finite-event history with a nonempty final market, two mature handoffs with actual consecutive outputs complete by
\[
 V_{\mathrm{cal}}\le\Psi_F^{\circ3}(t_*+1).
\]
After this handoff, write \(o_j\) for the root output times and \(L_j\) for the common waiting lengths, starting with the second recovery output. If the final market has \(n\) players, put \(d_0=2n-1\), \(V_j=o_j+d_0\), and \(Q_j=o_j+L_j\). Then \(V_0=V_{\mathrm{cal}}\), and
\begin{align}
 o_{j+1}&=o_j+L_j+c_j,
 &0<c_j&\le2J+2K-1, \label{eq:general-output-recursion}\\
 L_{j+1}&=F(L_j+c_j)\ge H+2L_j,
 &V_{j+1}-Q_j&\le U. \label{eq:general-maintenance-recursion}
\end{align}
From \(V_{\mathrm{cal}}\) onward, matching is correct outside \([Q_j,V_{j+1})\). For all legal instances, including an empty final market, and every integer \(T\ge0\),
\begin{equation}
 D_F(T;I)\le
 \min\{T,\Psi_F^{\circ3}(t_*+1)+U N_F(T)\}.
 \label{eq:general-wait-accounting}
\end{equation}
\end{sublemma}

\begin{proof}
\emph{Calibration and maintenance.} \Cref{lem:recovery} supplies the two actual consecutive mature outputs. \Cref{sec:proof-maintenance} gives their common waiting length and \cref{lem:maintenance} supplies the recurrences, fixed output offsets, and correct replay outside maintenance windows. Both lemmas apply to the general waiting rule \(F\), independently of \cref{thm:known}.

\emph{Counting windows in a prefix.} Since \(L_0\ge H=b_0\) and \(L_{j+1}\ge F(L_j)\), monotonicity yields \(L_j\ge b_j\). A window meeting the evaluation prefix \(\{1,\ldots,T\}\) starts at \(Q_j\le T\). As \(o_j\ge1\),
\[
 b_j\le L_j=Q_j-o_j\le T-1<T.
\]
Thus at most \(N_F(T)\) windows can contribute, each costing at most \(U\), including an unfinished last window. Charging one per round before \(V_{\mathrm{cal}}\) proves the bound for prefixes reaching calibration.

Earlier prefixes satisfy \(D_F(T;I)\le T<V_{\mathrm{cal}}\). For an empty final market, no cost occurs from \(t_*\) onward, and \(D_F(T;I)\le\min\{T,t_*-1\}\). Finally \(D_F(0;I)=0\), so the accounting covers every horizon.
\end{proof}
