# Supplementary material for: Decentralized Dynamic Stable Matching
Source: arXiv:2610.41912 source file (2026-11-06)
Supplement: Supplementary file 10 [file sweep-isolation.tex]

\subsection{Successful sweeps establish mature entry}
\label{sec:proof-sweep}

The BUS qualification interval clears earlier computations, and the sweep's isolated one-round gaps at BUS prevent new ones from starting. This isolation holds before success and is used in the recovery proof. A successful block then brings all other players to \SEEK{} and establishes the mature entry required by \cref{lem:mature}.

\begin{sublemma}[Sweep isolation and mature entry]
\label{lem:sweep}
Consider a history of \protocol{} reachable from the prescribed initialization, and let player \(z\) enter \SWEEP{} in global round \(b\).
\begin{enumerate}[label=(\roman*)]
  \item \emph{Isolation during a continuing scan.} Suppose \(z\) remains in this visit through round \(d\) and is accepted at every BUS action in rounds \(b,\ldots,d\). At the start of \(b\), after all round-start checks, every other present player is in \SEEK{} or \REPLAY{}, with \(\rho=0\) and no pending \WORK{} entry. Throughout \(b,\ldots,d\), all other players remain in \SEEK{} or \REPLAY{} and never schedule \WORK{}; in particular, none enters \SWEEP{} or produces an output. Population events and failed blocks are allowed.
  \item \emph{Mature entry after success.} If this visit completes an all-accepted block in round \(e\), and no population event occurs in round \(c=e+1\), then \(c\) is a mature entry with \(z\) as root. Population events during qualification and the scan, including at the start of round \(e\), are allowed.
\end{enumerate}
\end{sublemma}

\begin{proof}
\emph{Clearing earlier computations.}
Round-start states are taken after population events, pending mode changes, expiration, and qualification. Put \(v=b-J\). Since every action other than an accepted BUS proposal resets \(\rho\), even after saturation, qualification at \(b\) implies that \(z\) is accepted at BUS in
\begin{equation}
  v,v+1,\ldots,b-1.
  \label{eq:sweep-qualification}
\end{equation}
No other player can complete an AA pair or a successful block in this interval, since both require a final BUS acceptance. Thus no other \WORK{} entry is scheduled.

Any \WORK{} entry pending from \(v-1\) takes effect at \(v\), so all earlier \WORK{} invocations finish by \(v+J-1=b-1\). A competing sweep present at \(v\) reaches BUS by \(v+1\) and, if still present, returns to \SEEK{} by \(v+2\). Every other player's counter is reset in each qualification round, excluding new sweeps in \(v+1,\ldots,b\). Since \(J>2\), all other players are in \SEEK{} or \REPLAY{} at \(b\), with zero counters and no pending \WORK{}. Arrivals start in \SEEK{} with \(\rho=0\), and departures simply remove players.

\emph{Isolation during the sweep.}
The scan word \eqref{eq:sweep} leaves BUS only for isolated single rounds, including across failed-block restarts. Non-BUS rejections mark a block as failed without restarting it. Since \(z\) wins every BUS action, every other player's consecutive BUS-acceptance count stays at most one. Thus neither an AA handoff nor a new sweep qualification is possible, and all other players remain in \SEEK{} or \REPLAY{}. This proves (i) on every continuing prefix, regardless of eventual success.

\emph{Mature entry after success.}
On a BUS rejection, the player skips the block-completion test and leaves \SWEEP{} in the following round. Thus a visit completing a successful block at \(e\) has only BUS acceptances, and (i) applies with \(d=e\). No other output occurs: each old replay keeps its saved arm until it ends, and no seeker reenters \REPLAY{}. A player still replaying when its saved arm is visited is rejected. Every arm is visited by \(e-2\), so all old replays have ended by \(e-1\); later arrivals start in \SEEK{}.

The final two proposals are to BUS. In round \(e\), every other present player, including any new arrival, therefore proposes to BUS and is rejected. Each ends the round in \SEEK{} with a rejection recorded during its current visit, \(\rho=0\), and no pending \WORK{}. Since \(z\) wins against all these players, it is the highest-ranked player at BUS. With no population event at \(c=e+1\), its scheduled \WORK{} entry establishes the mature entry in \cref{def:mature}.
\end{proof}
